# Supplementary material for: Morphence-2.0: Evasion-Resilient Moving Target Defense Powered by Out-of-Distribution Detection
Source: arXiv:2206.07321 source file (2022-06-15)
Supplement: Supplementary file 1 [file appendix.tex]

\section*{Appendix}
\label{sec: appendix}

\subsection{Base Models Architectures}\label{subsec:base-models}
In Table \ref{tab:models}, we detail the architectures of MNIST-CNN and CIFAR10-CNN.
\begin{table}[h!]

 \begin{center}
    \scalebox{.80}{

   \begin{tabular}{|c|c|} 
   
   \hline
       
      \textbf{Base model} & \textbf{Architecture} \\ \hline
MNIST-CNN & \shortstack{$Conv2d(1, 32, 3, 1)+Relu$;
            $Conv2d(32, 64, 3, 1)+Relu$\\
            $max\_pool2d+dropout(0.25)+flatten$;
            $Linear(9216,128)+Relu$\\
            $dropout(0.5)+Linear(128, 10)$;
            $softmax(1)$}
         \\
         \hline

CIFAR10-CNN& $\shortstack{Conv2d(3,32,3,1)+
            BatchNorm2d(32)+
            ReLu;\\
            Conv2d(32,64, 3, 1)+
            ReLU+
        MaxPool2d\\
        Conv2d(64, 128, 3, 1)+
            BatchNorm2d(128)+
            ReLU\\
            Conv2d(128, 128, 3, 1)+
            ReLU+
            MaxPool2d+
            Dropout2d(p=0.05)\\
            Conv2d(128, 256,3,1)+
            BatchNorm2d(256)+
           ReLU\\
            Conv2d(256, 256, 3, 1)+
            ReLU+
            MaxPool2d\\
            flatten+Dropout(p=0.1)+
            Linear(4096, 1024)+
            ReLU\\
            Linear(1024, 512)+
            ReLU+
            Dropout(p=0.1)+
            Linear(512, 10)
            }$ \\ 
       \hline

   \end{tabular}}
 \end{center}
\vspace{2em}
 \caption{Base models architectures.}\label{tab:models}

\end{table}

\subsection{Attacks}\label{subsec:attacks}

\textbf{Fast-Gradient Sign Method (FGS)}~\cite{FGSM}: This attack is a fast one-step method that crafts an adversarial example. Considering the dot product of the weight vector $\theta$ and an adversarial example (i.e., $x' = x+\delta$), $\theta^\top x' = \theta^\top x + \theta^\top \delta$, the adversarial perturbation causes the activation to grow by $\theta^\top \delta$. Goodfellow et al.~\cite{FGSM} suggested to maximize this increase subject to the maximum perturbation constraint $||\delta||< \epsilon$ by assigning $\delta = sign(\theta)$. Given a sample $x$, the optimal perturbation is given as follows:
\begin{equation}
\label{eq:FGSM}
    \delta^\star = \epsilon . sign(\nabla_xJ(\theta, x, y_{target}))
\end{equation}

\textbf{Carlini-Wagner (C\&W)}~\cite{CW}: This attack is one of the most powerful attacks, where the adversarial example generation problem is formulated as the following optimization problem:
\begin{equation}
\label{eq:BIM}
\begin{array}{rrclcl}
    minimize \quad D(x,x+\delta)\\
    \textrm{s.t.} \quad f(x+\delta) = y_{target}\\
    \quad x+\delta \in [0,1]^n
\end{array}
\end{equation}
The goal is to find a small change $\delta$ such that when added to an image $x$, the image is misclassified (to a targeted class $y_{target}$) by the model but the image is still a valid image. $D$ is some distance metric (e.g $||.||_0$, $||.||_2$ or $||.||_\infty$). Due to the non-linear nature of the classification function $f$, authors defined a simpler objective function $g$ such that $f(x+\delta)=y_{target}$ if and only if $g(x+\delta)<0$. Multiple options of the explicit definition of $g$ are discussed in the paper ~\cite{CW} (e.g., $g(x')=-J(\theta,x',y_{target})+1$). Considering the $p^{th}$ norm as the distance $D$, the optimization problem is simplified as follows:
\begin{equation}
\label{eq:BIM}
\begin{array}{rrclcl}
    minimize \quad ||\delta||_p + c.g(x+\delta)\\
    \textrm{s.t.} \quad x+\delta \in [0,1]^n\\
\end{array}
\end{equation}
where c $>$ 0 is a suitably chosen constant.\\

\textbf{SPSA ~\cite{uesato2018adversarial}:} Simultaneous Perturbation Stochastic Approximation (SPSA) is an attack that re-purposes gradient-free optimization techniques into adversarial example attacks. They explore adversarial risk as a measure of the model’s performance on worst-case inputs. Since the exact adversarial risk is computationally intractable to exactly evaluate, they rather frame commonly used attacks (such as the ones we described earlier) and adversarial evaluation metrics to define a tractable surrogate objective to the true adversarial risk. The details of the algorithm are in~\cite{uesato2018adversarial}.

\textbf{Copycat~\cite{CopyCat18}}: Copycat is a learning-based method to attack a model and steal its knowledge. It considers an adversary that has no access to the training data or classification problem of the target model. However, it uses a surrogate model that has the same architecture of the target model. The process of Copycat is training the surrogate model on a large set of Random Natural Images (ImageNet and Microsoft COCO) labeled (hard-label) by target model. Copycat only uses the hard-labels, it is not necessary to know the probabilities of the target model. In this paper, we use a transformed set of the training data (i.e., MNIST and CIFAR10) of the target model instead of Random Natural Images, which makes the attack stronger and suitable for robustness evaluation in worst case scenarios.

\subsection{Attack Hyper-Parameters}
\label{hyper}
In Table \ref{tab:params}, we specify the parameters used for each studied attack.

\begin{table}[h!]

 \begin{center}
    \scalebox{.97}{

   \begin{tabular}{|c|c|} \toprule

      \textbf{Attack} & \textbf{Hyper-Parameters} \\ \hline
         FGSM &  \shortstack{$lb = 0$, $ub = 1$,\\ which indicate the lower and upper \\ bound of features. These two parameters are\\ specified only for MNIST dataset.}\\
         \hline

       PGD& \shortstack{$lb=0$, $ub=1$, with solver parameters:\\ ($\eta = 0.5$, $\eta\_min=2.0$, $max_{iter}=100$)}. \\
       \hline
      
      SPSA & \shortstack{$learning\_rate=0.01$,   \\$spsa\_samples=128$, $nb_{iter}=10$}. \\
       \hline

   \end{tabular}}
   \vspace{2em}
                 \caption{Attack Hyper-Parameters.}\label{tab:params}

 \end{center}

\end{table}
